# Supplementary material for: Backdoor Attack and Defense in Federated Generative Adversarial Network-based Medical Image Synthesis
Source: arXiv:2210.10886 source file (2023-07-16)
Supplement: Supplementary file 1 [file supplement.tex]

\section*{Supplementary Material}

\subsection{Responses to Reviewer’s Comments}

\subsection{Responses to Reviewer \# 1}

\paragraph{Comment 1.1}The FedDetect depends on the assumption that the poisoning images can easily overfit discriminating the trigger. Will this assumption always holds? We could relatively easy to train on a poisoned dataset with another GAN, which generate reversed labeled images. Such poison dataset could have similar distribution of the original dataset, and not easily overfit discriminating the trigger.
\paragraph{Response 1.1}When we stated the assumption in our submitted manuscript, we focused on the backdoor images with explicit triggers integrated into the training images. This focus was based on the prevalent existence of unintentional triggers commonly found in medical images, as depicted in Figure 2 of our revised submission. During our experiments, we observed the success of our attack through the degradation of both image fidelity and utility.

We thank reviewer 1 for raising this interesting scenario for the backdoor data. We tested this scenario and found that on the datasets used in this study, we consistently observed overfitting in various settings. Specifically, we model a strong attack by flipping the labels for the malicious client.  We launched experiments with a total number of clients ranging from 4, 6, 8 to 10 on the ISIC dataset. All clients randomly sampled an equal number of data points. One client is randomly chosen to be the malicious client for call cases. Except for the attacking strategy, all hyper-parameters and optimizers are kept the same as in the original paper. We examine the proportion of each local discriminator's ability to correctly classify fake images as fake. In this context, an overfitting discriminator is anticipated to demonstrate a greater capability in distinguishing fake images from real ones, resulting in a higher proportion of fake images correctly classified as fake. The results are shown in Fig 1. For better visualization, we smooth the proportion curve by running the average with a window size of 20. As shown, 
% \subsection{More Experiments Results.}

\newpage

\subsection{Training Details for Diagnostic Model}
\label{sup:clas}
\begin{table}[H]
\centering
\caption{The hyper-parameters investigated while training the classification models. Both the ISIC and the ChestX are trained over 20 epochs.}
\label{tab:1d-cnn}
\resizebox{0.9\linewidth}{!}{
\begin{tabular}{@{}cccc@{}}
\toprule
Hyper-parameter & Range Investigated  \\
\midrule
Seed & [1,2,3,4,5] \\
\#Real Sampled & [1,10,20,50,100,200,500] \\
Poison Size & [16,32,64] \\
Batch Size & [32]  \\
%  &  &  \\
\bottomrule
\end{tabular}
}
\end{table}

\begin{table}
\centering
\caption{Average Classification Accuracy (ISIC)}
\begin{tabular}{@{}ccccccccc@{}}
\toprule
\multirow{1}{*}{Settings} &
1 & 10 & 20 & 50 & 100 & 200 & 500  \\ 
\midrule
All Real $\uparrow$ & 0.50 & 0.53 & 0.50 & 0.54 & 0.60 & 0.72 & 0.75 \\
Vanilla $\uparrow$ & 0.73 & 0.74 & 0.75 & 0.76 & 0.77 & 0.79 & 0.79 \\
Attack 16 $\uparrow$ & 0.73 & 0.72 & 0.72 & 0.72 & 0.73 & 0.74 & 0.75 \\
Attack 32 $\uparrow$ & 0.62 & 0.65 & 0.63 & 0.66 & 0.67 & 0.69 & 0.70 \\
Attack 64 $\uparrow$ & 0.66 & 0.67 & 0.66 & 0.69 & 0.69 & 0.70 & 0.73 \\
Defense 16 $\uparrow$ & 0.73 & 0.73 & 0.73 & 0.73 & 0.75 & 0.76 & 0.78 \\
Defense 32 $\uparrow$ & 0.76 & 0.75 & 0.76 & 0.76 & 0.76 & 0.77 & 0.78 \\
Defense 64 $\uparrow$ & 0.66 & 0.68 & 0.69 & 0.70 & 0.74 & 0.76 & 0.80 \\
\bottomrule
\end{tabular}
\label{tab:isicDefense}
\end{table}

\subsection{Model Structure}
For image generation with GAN, we apply styleGAN-ADA generator structure. Its detailed structure can be found here~\cite{karras2020training}. For the discriminator, we apply the DCgan's architecture, which is outlined in the table below.
\label{sup:disc}
\begin{tabularx}{0.6\textwidth}{c|c}
\toprule
Layer & Details\\
\midrule
1 & Conv2D(channels, featues, 4, 2, 1), LeakyReLU\\
2 & Conv2D(featues, featues*2, 4, 2, 1), BN,  LeakyReLU\\
3 & Conv2D(featues*2, featues*4, 4, 2, 1), BN,  LeakyReLU\\
4 & Conv2D(featues*4, featues*8, 4, 2, 1), BN,  LeakyReLU\\
5 & Conv2D(featues*8, featues*16, 4, 2, 1), BN,  LeakyReLU\\
6 & Conv2D(featues*16, featues*32, 4, 2, 1), BN,  LeakyReLU\\
7 & Conv2D(featues*32, 1, 4, 2, 0),  Sigmoid\\
\bottomrule
\end{tabularx}
